# Supplementary material for: Occam's Razor for Self Supervised Learning: What is Sufficient to Learn Good Representations?
Source: arXiv:2406.10743 source file (2024-06-15)
Supplement: Supplementary file 1 [file appendix.tex]

\section{Computationally Friendly SOlution to Non-Parametric VICReg}
\label{appendix:friendly}

{\bf Computationally friendly solution.}~Before concluding this section we ought to recall that \cref{eq:VICReg_optimal}, which needs to be decomposed to obtain $\mZ^*_{\alpha,\gamma}$ is a dense $N \times N$ matrix e.g. as follows
\begin{lstlisting}[language=Python,escapechar=\%]
L = ch.diag(G.sum(1)) - G # Laplacian matrix %\lsComment{$\mL$}% in Eq. %\lsComment{\ref{eq:VICReg_optimal}}%
Lam, P = ch.linalg.eigh(torch.eye(N) - 1 / N - (gamma / alpha) * L) #equals to %\lsComment{(\ref{eq:VICReg_optimal})}%
Z_star = P[:, -K:] * ((Lam[-K:] * N).sqrt()) # equals to %\lsComment{$\mZ^*$ of Thm. \ref{thm:VICReg_optimal}}%
min_L = alpha * (K - Lam[-K:].norm().square()) # equals to %\lsComment{$\min \mathcal{L}_{\rm vic}$ of Thm. \ref{thm:VICReg_optimal}}%
\end{lstlisting}
However, we can equivalently find the optimal VICReg solution $\mZ^*_{\alpha,\gamma}$ only as a function of $\mL$ which is sparse e.g. for SSL $\mL$ contains $2N$ nonzero entries, and for supervised settings with $C$ balanced classes, $\mL$ contains $N^2/C$ nonzero entries. To do so, notice in \cref{eq:VICReg_optimal} that the left term $\mI-\frac{1}{N}\mathbf{1}\mathbf{1}^T$ mostly acts to ensure that the found eigenvectors with nonzero eigenvalues have $0$ mean. Instead, we can achieve the same goal by defining the following {\em sparse and symmetric} matrix
\begin{align}
    \begin{pmatrix}
    0 & \mathbf{1}^T\\
    \mathbf{1} & \mI - \frac{\gamma}{\alpha}\mL
    \end{pmatrix}\in\mathbb{R}^{ (N+1)\times(N+1)},\label{eq:sparse_J}
\end{align}
and by taking the top $[2:K]$ (and not $[1:K-1]$ as with \cref{eq:VICReg_optimal}) eigenvectors. In short, while \cref{eq:VICReg_optimal} was adding a connection from each node of the graph to all others, \cref{eq:sparse_J} introduces a new node to the graphs and connects it to all others, akin to the Hubbard-Stratonovich transformation \citep{hirsch1983discrete}. The great advantage of \cref{eq:sparse_J} is the sparsity of the matrix allowing it to be easily stored and for which there exists efficient routines to rapidly obtain the top eigenvectors, even for large $N$. One popular solution is the Locally Optimal Block Preconditioned Conjugate Gradient \citep{knyazev1987convergence} which only needs to evaluate matrix-vector products.
